# Supplementary material for: Deep Proxy Causal Learning and its Application to Confounded Bandit Policy Evaluation
Source: arXiv:2106.03907 source file (2024-06-18)
Supplement: Supplementary file 1 [file symbols.tex]

\begin{tabular}{l|l}
    \hline
     $A$, $\mathcal{A}$, $\prob{A}$, $a$ &  random variable, space, probability distribution, realization of treatment  \\ \hline
     $Y$, $\mathcal{Y}$, $\prob{Y}$, $y$ &  random variable, space, probability distribution, realization of outcome  \\ \hline
     $W$, $\mathcal{W}$, $\prob{W}$, $w$ &  random variable, space, probability distribution, realization of outcome-proxy  \\ \hline
     $Z$, $\mathcal{Z}$, $\prob{Z}$, $z$ &  random variable, space, probability distribution, realization of treatment-proxy  \\ \hline
     $U$, $\mathcal{U}$, $\prob{U}$ &  random variable, space, probability distribution of confounder  \\ \hline
     $f_{\mathrm{struct}}$ &  structural function \\ \hline
     $h^*$ &  true bridge function \\ \hline
     
\end{tabular}
